# Supplementary material for: Theoretical investigation on the formation of ethylene on a gold surface
Source: arXiv:2509.22835 source file (2025-09-26)
Supplement: Supplementary file 1 [file SI_EthylOnAu.pdf]

# Supporting Information: Theoretical investigation on the formation of ethylene on a gold surface.

Tim Schrader,<sup>†</sup> Alen Shaji,<sup>†</sup> Christin David,<sup>‡</sup> and Eva Perlt<sup>\*,†</sup>

<sup>†</sup>*Otto Schott Institute of Materials Research (OSIM), Faculty of Physics and Astronomy,  
Friedrich Schiller University Jena, Löbdergraben 32, 07743 Jena, Germany*

<sup>‡</sup>*University of Applied Sciences Landshut, Am Lurzenhof 1, 84036 Landshut*

E-mail: [eva.von.domaros@uni-jena.de](mailto:eva.von.domaros@uni-jena.de)

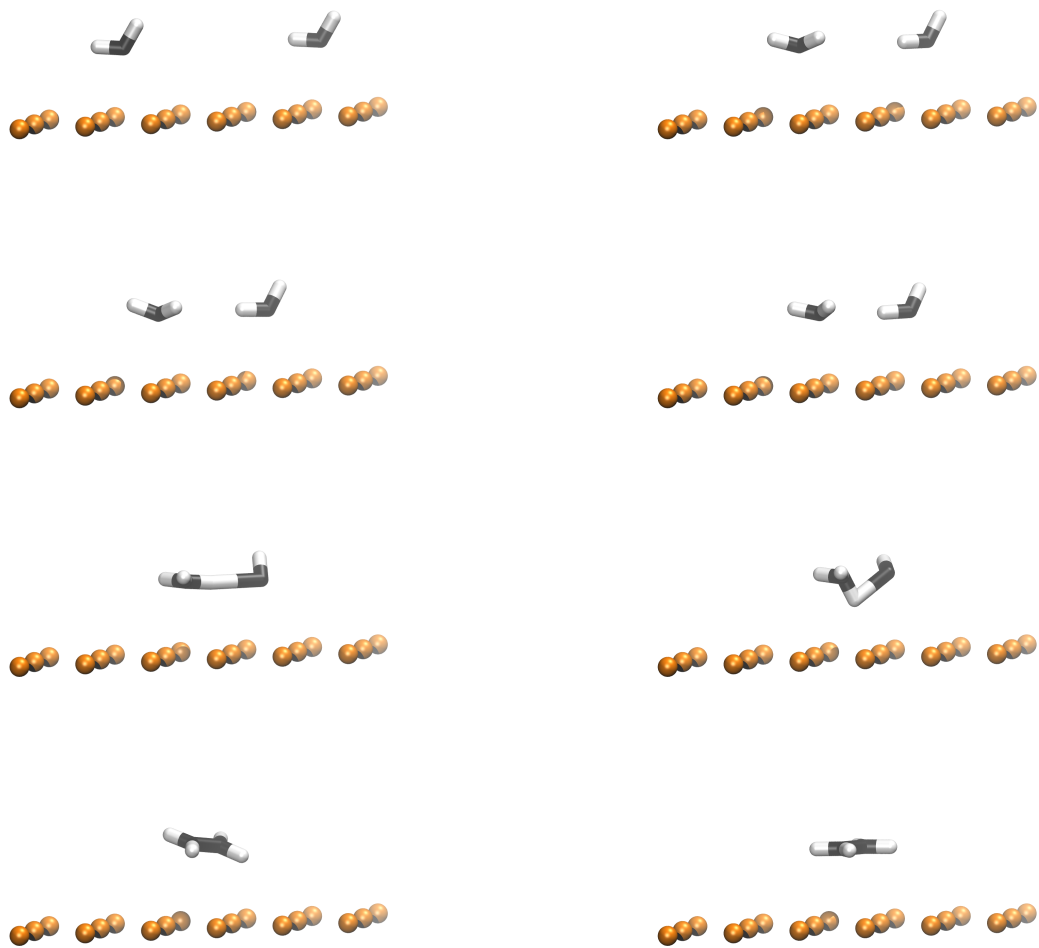

Figure S.1: Snapshots along the reaction coordinate on one layer of gold. Shown are educts (top left), reaction coordinates five (top right), six (second row left), seven (second row right), nine (third row left), eleven (third row right), 13 (bottom left) and the product geometry (bottom right).

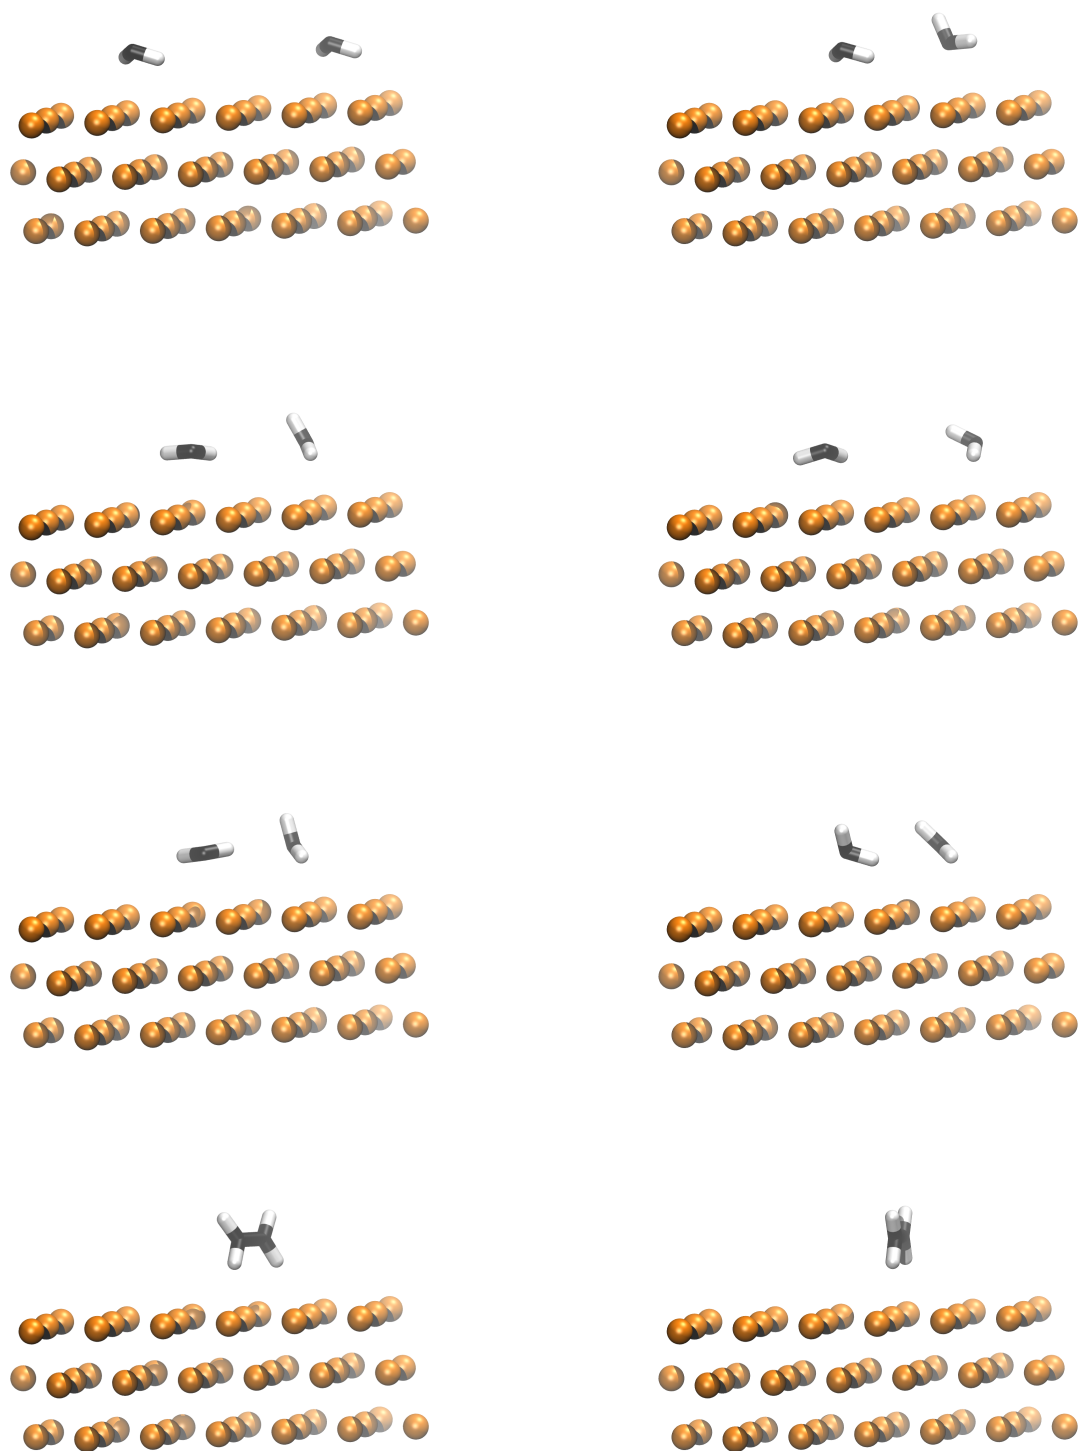

Figure S.2: Snapshots along the reaction coordinate on three layers of gold. Shown are educts (top left), reaction coordinates five (top right), six (second row left), seven (second row right), nine (third row left), eleven (third row right), 13 (bottom left) and the product geometry (bottom right).
